# Supplementary material for: Laser-induced frequency tuning of Fourier-limited single-molecule emitters
Source: arXiv:2005.12199 source file (2020-05-25)
Supplement: Supplementary file 1 [file Supporting_Information.pdf]

# Supporting Information

Sublimation growth of DBT:DBN single crystals ........ 1
Preparation of DBT:Ac nanocrystals ........ 2
Optical microscopy (DBT:DBN) ........ 2
Optical microscopy (DBT:Ac) ........ 3
Measurements of DBT:Ac nanocrystals ........ 4
Shift dependence of power and pump laser wavelength ........ 4
Measurement of the photon statistics: single photon purity ........ 6
Measurements of DBT:DBN single crystals ........ 7
Single-molecule trajectories and inter-molecular heterogeneity ........ 7
Power law behavior of individual trajectories ........ 9
Spectral shift power dependence in DBT:DBN ........ 9
Background fluorescence ........ 9
Dibenzoterrylene in polycrystalline naphthalene ........ 11
Quantum chemistry calculations ........ 13
Calculations on isolated molecules ........ 13
Energies of the excited electronic states of DBT ........ 13
Calculations of locally excited (LE) and charge-transfer (CT) states ........ 14
Electronic states and transitions of bimolecular DBT/DBN system ........ 15
Electronically excited states of DBT:Ac system ........ 15
Recovery of neutral DBT ........ 19
*Case A: Spontaneous filling of the hole* ........ *19*
*Case B: Recovery of neutral DBT with the aid of optical excitation.* ........ *19*
Consistency of the model with experiments ........ 20
Supplementary references: ........ 22

## Sublimation growth of DBT:DBN single crystals

2,3-dibromonaphthalene (DBN) used in this work was purchased from Ark Pharm Inc. High-quality single crystals of zone-refined DBN doped with dibenzoterrylene (DBT) molecules were obtained by co-sublimation at ~ 0.2 bar of argon gas. To prevent perturbations from the convection flow in the sublimation chamber, the sublimator was kept horizontal during growth. The sublimation-grown crystals develop along the (*a*,*b*) plane as thin mm-sized plates or flakes, with a typical thickness of few microns along the *c*-axis.

## Preparation of DBT:Ac nanocrystals

Nanocrystals (NCs) of anthracene (Ac) doped with single-molecule concentration of dibenzoterrylene (DBT) are grown by injecting 100 µL of 4:$10^7$ mixture of 1 mM DBT-toluene and 5 mM Ac-acetone solutions into 2 mL of sonicating milliQ water. After 30 min of sonication, solvents are completely dissolved and DBT:Ac NCs are formed as aqueous suspension (for more details see ref. [S1]). The nanocrystals are then deposited on the substrate via drop-casting of ~10 µL of the suspension followed by dessication. In particular, the substrates employed in the experiment are simple glass coverslips and coverslips coated with sputtered gold (film-thickness of ~200 nm). After the deposition, NCs are protected from sublimation by spin-coating a ~200 nm thick layer of polyvinyl alcohol (PVA).

Solvents, Ac and PVA were purchased from Sigma-Aldrich, water was deionized by a Milli-Q Advantage A10 system (resistivity of 18.2 MΩ×cm at 25°C), and DBT was purchased from Mercachem.

## Optical microscopy (DBT:DBN)

All single-molecule measurements with DBT:DBN crystal were done at 1.2 K in a home-built liquid-helium bath cryostat. Single crystals of DBT:DBN were optically attached to a glass substrate containing interdigitated gold markers previously deposited by lithography, which served to locate different parts of the single crystal in consecutive experiments. All pump excitation experiments on DBT:DBN were performed on the crystal parts which were in contact with the glass substrate.

Single DBT molecules were excited by a tunable continuous wave Ti:Sapphire laser (M Squared) at around 756.7±0.2 nm. This laser is denoted in the main text as a probe (laser) beam. The frequency range of typically 10 GHz was scanned with 1000 points and 5 ms integration time per point, with a typical power of 0.3 – 0.7 µW focused on the sample. The output of the laser was continuously monitored by an external Fabry-Perrot cavity. The response of this cavity was used to monitor the laser frequency drift in real time and to compensate for a small non-linearity of the frequency scan.

A second, more intense (pump) laser beam was used to induce spectral shifts in DBT:DBN crystals. The laser light was produced by a Coherent ring laser, operated with Rhodamine 101 (640) dye and pumped with a 532 nm solid state laser. The operating wavelength of the pump laser was at around 631 nm, and a typical power focused on the sample was 10 µW – 5 mW, depending on the experiment and on the spectral shifts to induce. In all experiments the sample was scanned with either only probe laser (756.7 nm) or simultaneously with both pump (631 nm) and probe lasers focused on the sample.

The sample was scanned in a confocal epi-fluorescence arrangement using a scanning mirror (Newport, FSM-300-01). A λ/4 wave plate was used to produce a circularly polarized beam for more efficient excitation of single DBT emitters. The fluorescence light was collected by a cryogenic objective (Microthek, NA = 0.8) and detected by a single-photon counting module

(Excelitas Single-Photon Counting Module, SPCM-AQRH-16) with a set of filters (Chroma HQ760LP and Semrock FF02-809/81) in the detection path.

## Optical microscopy (DBT:Ac)

The optical characterization of individual DBT molecules in Ac NCs was performed with a home-built scanning fluorescence confocal microscope. All measurements were done at about 3.5 K, with the sample in a closed-cycle helium cryostat (Cryostation by Montana Instruments). The transition linewidth of individual molecules was measured under confocal resonant excitation, with a  CW distributed feedback diode laser (Toptica, LD-0785-0080-DFB-1), named 'probe' in the paper, which is centered at 784.6 nm and can be scanned continuously in frequency over a range of 800 GHz. Frequency shifts of molecules' emission were generally induced in off-resonant configuration by using a CW external-cavity diode laser (Toptica, DLX110), named 'pump' in the paper, centered at 767 nm and operated at higher power (also in confocal mode). In particular, the laser frequency can be tuned through fine tilting of the Bragg grating of the diode source, enabling mode-tuning within about ±4 nm around the central value. Laser-induced shifting was also performed by using the probe laser operated at higher power. All laser sources were fiber-coupled and linearly polarized by means of a half-wave plate in the excitation path to allow for optimal coupling to the single molecule's linear dipole. The excitation light was focused onto the sample by a glass-thickness-compensation air objective (OptoSigma 50x, N.A.=0.67, WD=10.48mm) and scanned over the sample by a telecentric system and a dual-axis galvo-mirror. The Stokes-shifted fluorescence was hence separated from the excitation light through a dichroic mirror (Semrock FF776-Di01) and a long-pass filter (Semrock RazorEdge LP02-785RE-25), and detected by either an EMCCD camera (Andor iXon 885, 1004×1002pixels, pixel size 8 mm×8 mm), for measuring fluorescence space-maps and spectral properties, or by a SPAD (SPCM-AQRH-14-TR by Excelitas). A converging lens was inserted in the excitation path, just before the dichroic mirror, to switch between confocal and wide-field illumination.
For the anti-bunching measurement shown hereafter, we employed a Hanbury-Brown and Twiss configuration, based on a fibered beam-splitter, two fiber-coupled SPADs (SPCM-800-14-FC by Excelitas) and a time-correlated single-photon counting (TCSPC) card (PicoHarp 300 by PicoQuant). Fiber-coupling of the single-molecule fluorescence was achieved by means of an adjustable fiber-collimator and a free-space telescope for mode-matching.

## Measurements of DBT:Ac nanocrystals

### Shift dependence of power and pump laser wavelength

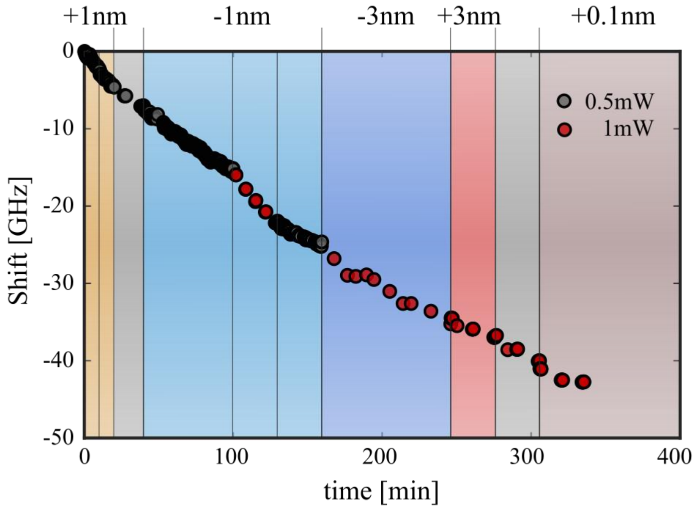


*Figure S1: 0-0-ZPL transition shift induced on the same single molecule by a succession of "pump" laser bursts with different characteristics (wavelength and illumination power). The data-points are the ZPL resonant frequencies obtained from a Lorentzian fit to the excitation spectra. Data-points colors refer to the pump power value, whereas the temporal color-bands indicate the pump wavelength with respect to the most efficient excitation rate of the 0-1 transition, labeled in gray and corresponding to the pump at 767.8nm.*

In Fig. S1 the entire dynamics of the ZPL-transition frequency shift for an individual DBT molecule in an Ac-nanocrystal is reconstructed by monitoring its position after several consecutive burst exposures, operated with different parameters (illumination power and wavelength). The temporal colored bands indicate the pump wavelength value, according to the labeling on the right. Furthermore, colors of the dotted data refer to the two employed pump powers, one double (red) the other (black). This latter parameter change can be used as term of comparison: while the induced-shift dynamics is clearly dependent on the pump power (see also Fig. 2a in the main text), it is not visibly sensitive to wavelength. Consequently, we can state that the photochemistry process responsible for the charge separation and the Stark shift does not result from excitation of the DBT molecule under single-molecule investigation. Indeed, the spectral band explored in the measurements reported in Fig. S1 corresponds to very different pumping efficiencies for a given illumination power. By comparison with a reference excitation spectroscopy of the 0-1 transition obtained for a different molecule (Fig. S2), the excitation wavelengths labelled in gray in Fig. S1 correspond to the strong peak at 764.7 nm, hence to the maximum excitation efficiency. The wavelength labelled in orange is instead associated to the plateau between the two resonance peaks, hence to an excitation efficiency reduced by more than one order of magnitude, while for 3 nm on

the red (red band), we are close to the secondary resonance. Moreover, on the blue of the main peak it is established that no relevant resonances are present within 7 nm shift [S2] (not shown).

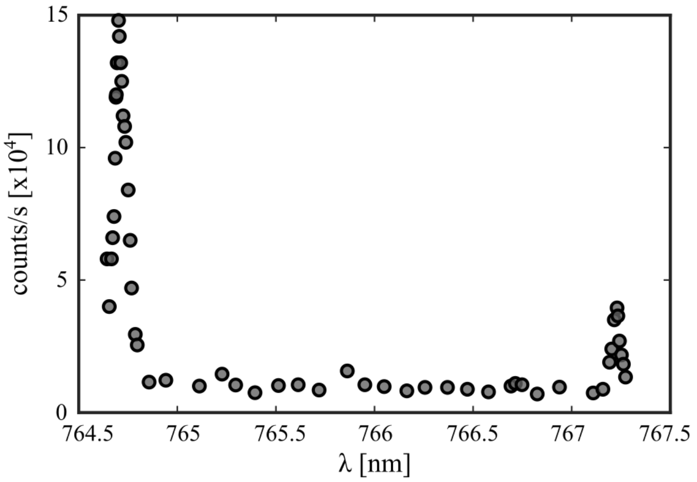


*Figure S2. Excitation spectroscopy performed with the "pump" laser around the 01-ZPL transition: recording the spectrally integrated fluorescence intensity gives access to the pumping efficiency as a function of illumination wavelength. The reported spectrum is not measured for the same molecule of Fig. S1, and in particular the main excitation peak in this case was shifted by around 3 nm to the blue with respect to the molecule of Fig. S1. However, we have found evidence that the level scheme is almost rigidly shifted by the inhomogeneous broadening. Our findings are in substantial agreement with ref.[S2].*

Despite this big variation on pumping efficiency, the laser-induced shift recorded in Fig. S1 is not correspondingly affected by the difference in the excitation efficiency of the DBT molecule under investigation, as a function of the pump laser frequency. This is a relevant indication that the light-induced shift does not depend strongly on the target molecule's ZPL-transition.

## Measurement of the photon statistics: single photon purity

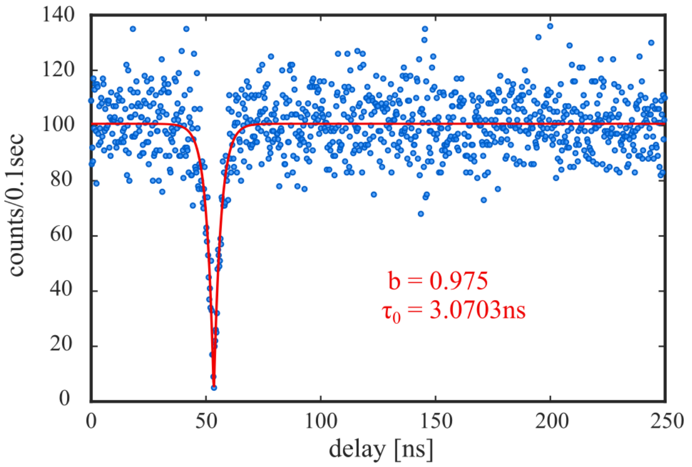


*Figure S3. Anti-bunching measurement for fluorescence collected from an individual DBT:Ac nanocrystal under illumination with "pump" laser at 767 nm, evaluated as a histogram of the differential arrival times of the photons on two avalanche photodiodes in a Hanbury-Brown and Twiss configuration. The second-order autocorrelation function at zero delay is inferred by the best fit (red line) to the experimental data (blue dots), yielding $g^{(2)}(0)=1-b=0.03\pm0.03$. In particular, the fit function is $g^{(2)}(t) = A(1 - be^{-|t-t_0|/\tau})$, with A normalization factor, b anti-bunching dip depth, $t_0$ a time delay and $1/\tau$ accounting for the excitation and spontaneous emission rate.*

In Fig. S3 we show a representative example of anti-bunching measurements of an individual DBT:Ac nanocrystal. The data points are recorded under off-resonant excitation (767 nm). The second-order autocorrelation function at zero delay inferred by the fit to the experimental data yields $g^{(2)}(0)=1-b=0.03\pm0.03$, which proves the high purity of the single-photon emission. This result is not in contradiction with the measurements reported in the main text (Fig. 2), where we see a background comparable to the signal intensity. Indeed, shift measurements are performed with a strong illumination power (exciding by more than one order of magnitude the saturation level), which is able to excite other, more weakly coupled molecules. The latter are molecules without narrow lines, or with narrow lines at different wavelengths and/or spatially close to the one under investigation. With respect to the last "background source", a relevant gain is obtained also thanks to the spatial selection introduced by fiber-coupling.

# Measurements of DBT:DBN single crystals

## Single-molecule trajectories and inter-molecular heterogeneity

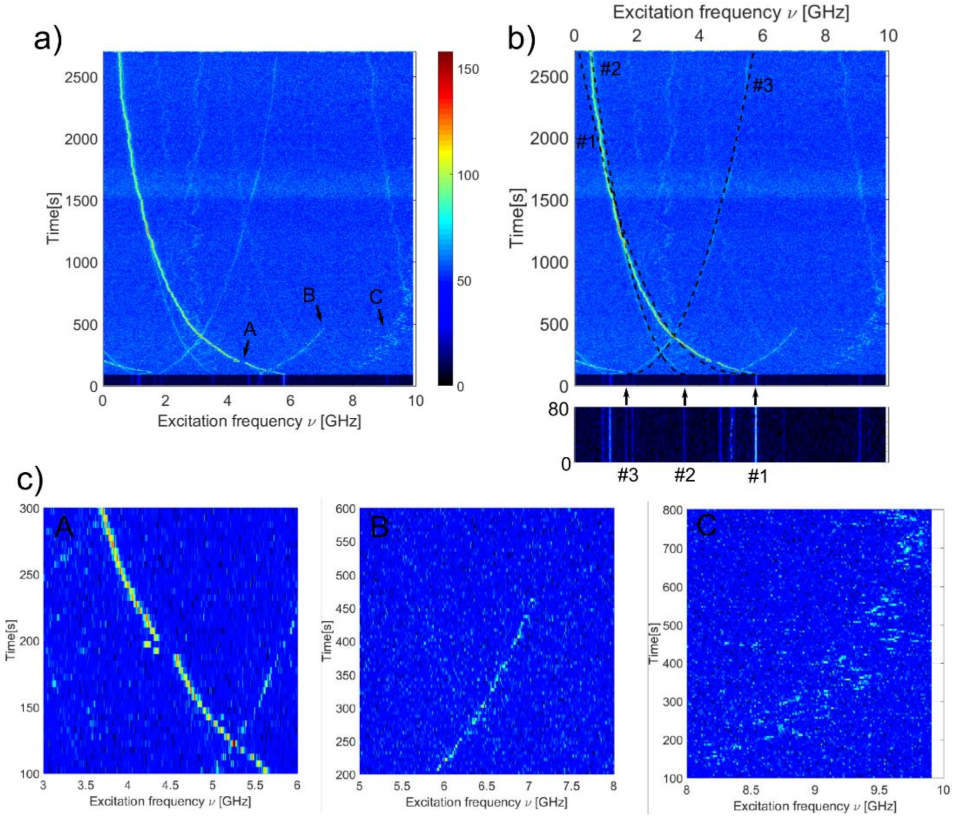


*Figure S4. a) Single-molecule fluorescence excitation spectrum of DBT molecules in 2,3-DBN recorded in real time during exposure to a pump beam (631 nm, 45 µW). Several ZPLs are visible showing different response to the pump beam. Highlighted events A-C are shown in (c). The dark blue background at the bottom indicates line scans without the pump beam. The probe beam was continuously scanned at 756.7 nm (0.7 µW). Color bar: counts per 5 ms. b) Power law fits for three molecules, indicated with arrows; molecule #1 (α=0.36, B=-340 MHz), molecule #2 (α=0.49, B=-60 MHz), and molecule #3 (α=0.47, B=100 MHz). The coefficients α and B are as in eq. (1) of the main text. Note that molecule #1 has the largest shift, but also the largest departure from the power law fit. c) Typical examples of a smaller spectral jump, possibly influenced by a nearby charge diffusion (A), large spectral jump or photobleaching event (B) and large and fast spectral diffusion with fast random jumps (C).*

DBT:DBN single crystals are prepared by a co-sublimation method, using zone-refined DBN. This method is considered to produce molecular crystals of highest quality and purity. Furthermore, using these crystals with relatively high concentration of well-embedded DBT molecules, we can locally sense charging events, charge migration and fluctuations in electric field buildup. As each molecule is embedded in a slightly different environment, the response of individual molecules may differ. Figure S4 illustrates this on a set of several molecules. Apart from fairly stable

trajectories in molecules #1, #2, and #3, one can discern other types of trajectories and local behaviors. For example, molecule #1 exhibits a small spectral jump (labelled as A in Fig. S4c) for ~ 10 s, which is likely an evidence of a nearby charging event. Event (B) highlights a molecule that suddenly photobleaches or undergoes a large spectral jump out of the frequency scan window (10 GHz). Trajectory (C) is from a spectrally unstable molecule that is seeing more frequent local perturbations due to local charge dynamics.

## Power law behavior of individual trajectories

Figure S4b shows power law fits to three long trajectories presented in Fig. S4a. As can be seen, all molecules do not display the same electric field change, and their trajectories are quantitatively different. Furthermore, power law functions cannot fully describe the behavior of all individual molecules, but it is a fairly good approximation on larger timescales of up to 1 h. For example, molecule #1 in Fig. S4 shows the largest response to the pump beam, but its behavior is not well-fitted by a power law. On the other hand, molecules #2 and #3 show a fairly good match with a power law behavior and their fitting parameters are very similar, even for longer timescales.

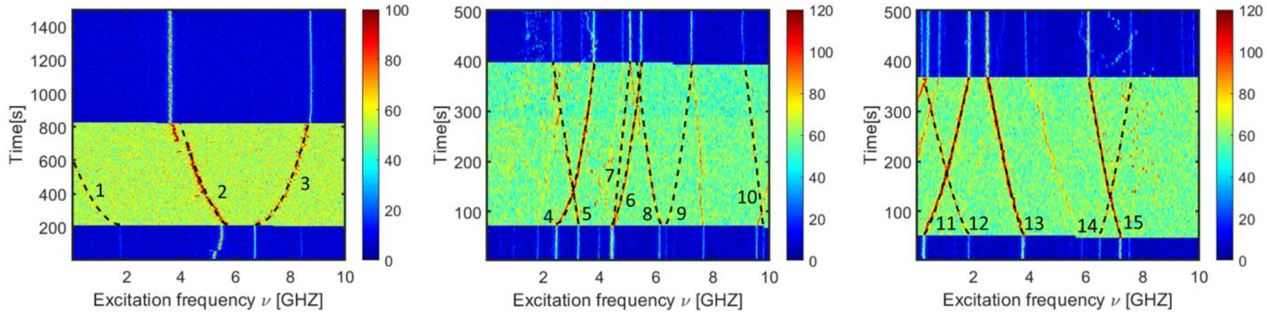


| No | 1 | 2 | 3 |
|---|---|---|---|
| B (MHz) | - 65 | -19 | 80 |
| α | 0.55 | 0.7 | 0.5 |

| No | 4 | 5 | 6 | 7 | 8 | 9 | 10 |
|---|---|---|---|---|---|---|---|
| B (MHz) | 60 | -2.8 | 25 | 1.8 | -15 | 16.5 | -2 |
| α | 0.54 | 1.0 | 0.65 | 1.0 | 0.7 | 0.7 | 1.0 |

| No | 11 | 12 | 13 | 14 | 15 |
|---|---|---|---|---|---|
| B (MHz) | 21.5 | -21.5 | -12.5 | 11.5 | -11.5 |
| α | 0.75 | 0.75 | 0.8 | 0.8 | 0.8 |

*Figure S5. Examples of 15 single-molecule trajectories, recorded at different points on a DBT:DBN crystal. The trajectories are fitted with a power law equation, $\nu = \nu 0 + B \cdot (t/t_0)^{\alpha}$, where $t_0 = 1$ s. The table includes fitted parameters B (MHz) and α for all 15 molecules. The pump excitation power was in all experiments ~ 50 µW at 631 nm. Color bars: counts per 5 ms.*

Despite the mentioned heterogeneities that are intrinsic to molecular systems perturbed with charging events at 1.2 K, we still find many molecules “well-behaving” in the pump beam. Figure S5 shows the examples of 15 single-molecule trajectories obtained on 3 different locations in a DBT:DBN crystal. All these trajectories (5 – 10 min long) are fitted well with a simple power-law equation. What is interesting to note is that up to several molecules in each scan can be fitted with very similar parameters B and α (e.g. molecules 11-15 in scan 3, Fig. S5), indicating that these DBT emitters experience very similar local electric fields. We find parameter α mostly having values between 0.5 – 1.0, where the lower α designates faster initial change in resonant frequency of a molecule and α = 1 means linear time dependence.

ZPLs of individual molecules do not drift or jump after the pump beam is switched off, as shown in Fig. S6. In this example the ZPL was tuned with a fairly low power of the pump beam (43 µW). As shown in Fig. 2 of the main text, the ZPL lines remain stable and can be shifted much faster with more intense (6 mW), shorter pump pulses (1 – 3 s). This holds for a large majority of single emitters and indicates that charge reconfiguration in the crystal upon pump illumination is almost instantaneous, but it does no longer affect the frequency of the optical transition after the pump beam has been switched off. The latter observation indicates long recombination times and large electron-hole separations in the sample.

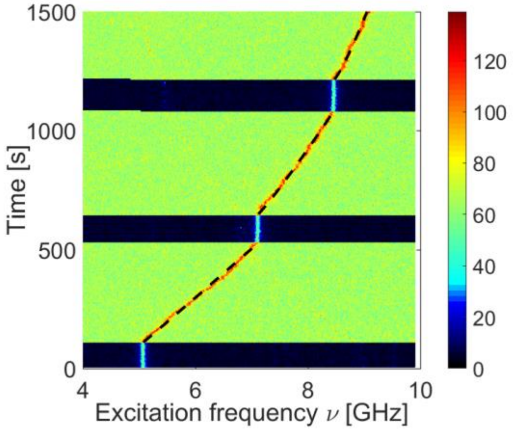


*Figure S6. Start-stop experiment with alternating pump excitation (on/off), for DBT in 2,3-DBN. The pump beam excitation was 43 µW at 631 nm, whereas the probe beam (0,7 µW) was continuously scanned at 756.7 nm. Color bar: counts per 5 ms. Dashed lines represent power law fits to the data, with B = 5.2 MHz, and $\alpha_1$=0.99 (bottom fit), $\alpha_2$=0.92 (middle fit), $\alpha_3$=0.84 (top fit).*

## Spectral shift power dependence in DBT:DBN

We have tested the behavior of individual emitters to increasing illumination powers of the pump beam. Figure S7 illustrates behavior of two emitters (#1 and #2) at three different powers, normalized to the dose of radiation. At 47 µW of pump illumination, the rate of shift change decays in time due to the power law behavior. Increasing of the pump power leads to further increase of spectral shifts and has close-to-linear power dependence. i.e., similar power-law trend is present when the shifts are rescaled to the dose of the pump beam.

## Background fluorescence

Background fluorescence in both DBT:Ac and DBT:DBN originates from fluorescent molecules that are excited with the pump beam. In the latter case, the contribution is largely due to the non-resonantly excited background molecules. The measured signal has close to linear power dependence (Fig. S8) indicating that we do not reach saturation of background signal at high excitation powers (above 1 mW).

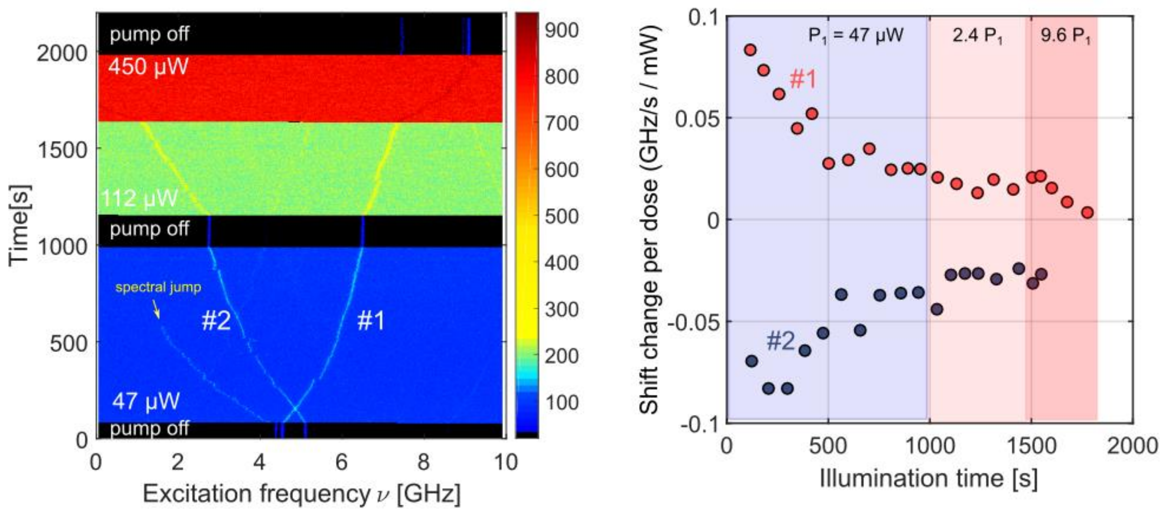


*Figure S7. Left: Single-molecule fluorescence excitation spectrum of DBT molecules in 2,3-DBN recorded in real time with different pump beam excitation powers at 631 nm (47 µW, 112 µW, and 450 µW). Two stable ZPLs (#1 and #2) are visible showing fairly similar response to the pump beam. The black background in the image indicates line scans without the pump beam. The probe beam was continuously scanned at 756.7 nm (0.7 µW). Color bar: counts per 5 ms. Right: Shift changes for molecules #1 and #2 shown in the left image, plotted in real time. The color-coded zones denote regions of different pump power. The spectral jump indicated with a yellow arrow may be a signature of a discrete ionization or trapping event.*

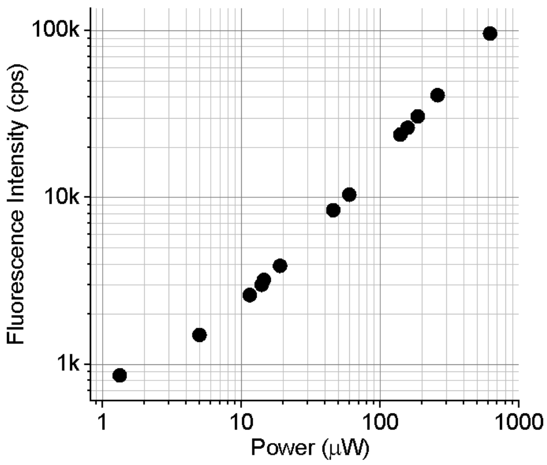


*Figure S8. Fluorescence background signal change with excitation power of the pump beam at 631 nm. The background signal originates from many excited DBT molecules in 2,3-DBN single crystal.*

We also observed that spectral shifts can be controlled by changing the polarization of the pump beam, affecting in this way the amount of excited DBT molecules (Fig. S9). The largest spectral shifts were obtained for the maximum of fluorescence background signal, proving that larger

number of excited DBT molecules leads to greater charge generation and, consequently, larger spectral shifts.

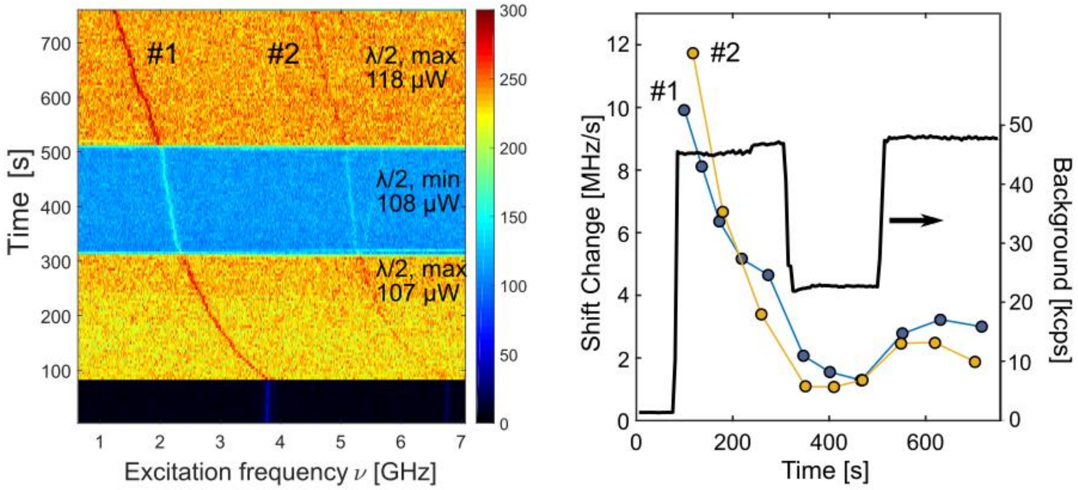


*Figure S9. Left: trajectories of two DBT molecules (#1 and #2) in DBN, whereby the polarization of the pump beam is varied with a λ/2 wave plate. The polarization state of the pump beam was adjusted in such a way that the background signal alternated between maximum (~47 kcps) and minimum (~22 kcps). To excite a larger number of molecules, the pump and the probe beam were previously circularly polarized with a λ/4 wave plate. Color bar: counts per 5 ms. Right: the average change of the spectral shifts in time for molecules #1 (blue circles) and #2 (red circles).*

## Dibenzoterrylene in polycrystalline naphthalene

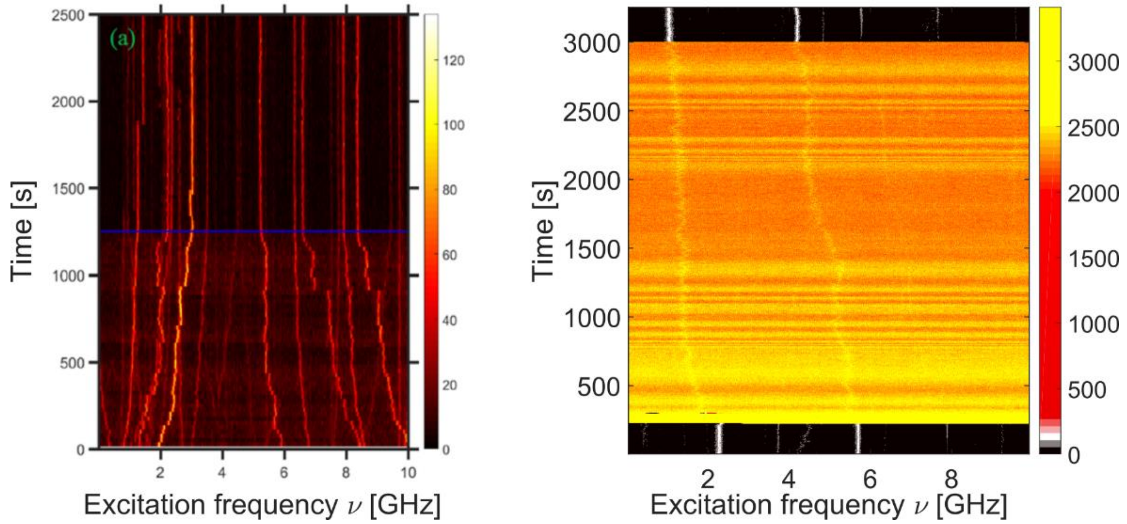


*Figure S10. Tunable spectral shifts of DBT in polycrystalline naphthalene, with pump excitation at 570 nm (left) and 631 nm (right). Color scale: counts per 5 ms.*

Spectral shifts of DBT in polycrystalline naphthalene can be induced with a pump beam of broad excitation range. In this example, we have used a tunable pump laser at several wavelengths in a

range of 570 – 635 nm. The ZPLs are photostable (no photobleaching or large spectral jumps) and the spectral shifts obtained are, on average, lower than in DBT:DBN and DBT:Ac systems, typically up to 1 GHz/mW per 1 hour of illumination. Spectral diffusion in this system is also more pronounced, with molecules changing the direction of their shifts in real time. The background signal has oscillating behavior (right panel). This pronounced background time-dependence is most likely due to the change in the refractive index of a crystal, induced by migration of charges – an effect typically observed in photorefractive materials.

## Quantum chemistry calculations

Quantum chemistry calculations were done in order to provide information about energies and character of electronically excited states in DBT/DBN and DBT/Ac crystalline systems. Performed calculations required big computer memory and were done by using the TDDFT/B3LYP method with 6-31G(d,p) or 3-21G bases. Theoretical calculations do not guarantee the same precision as the experimental data and thus should be treated with some caution. Calculations of electronic states in studied bimolecular systems (DBT:Ac and DBT:DBN) were performed for Ac and DBN molecules in their real crystal geometries. Embedding sites of DBT in both crystals were already optimized in our previous works [S3, S4]. Different substitution sites led to slightly different energies of the electronic states of DBT molecules embedded in DBN and Ac crystals.

### Calculations on isolated molecules

Tables S1 provides useful information about excitation energies of isolated DBT, DBN, and Ac molecules. The calculated lowest energy transitions (ΔE) agree well with the experimental values. Electron affinities (EA) and ionization potentials (IP) of isolated molecules shown in Table S1 can be used as useful descriptors of electron and hole stabilities, as they determine the polarization energies of created charges in the studied systems.[S5] Based on the values of electron affinities and ionization potentials, the activation energy needed to put the system into a conducting state can be estimated.[S5, S6] According to this empirical description, energy levels of electrons and holes on DBT (i.e., $DBT^-$ and $DBT^+$) will be in between the energy levels of charged host molecules (e.g., $Ac^+$ and $Ac^-$). DBT impurities will thus behave as traps for electrons and holes in both DBN and Ac. Therefore, the activation energy needed to drive the system into photoconducting state will decrease (from, e.g., 3.9 eV for pure anthracene crystal). This empirical interpretation of Karl and Silinsh is confirmed with our quantum chemistry calculations, as elaborated below in more details.

*Table S1. Isolated DBT, DBN and Ac – excitation energies (ΔE), ionization potentials (IP) and electronic affinities (EA). TDDFT/B3LYP/6-31G(d,p) results.*
*Note that IP (DBT) < IP(Ac) < IP(DBN), and EA (DBT) > EA(Ac) >EA(DBN).*

| | ΔE [eV] | IP [eV] | EA [eV] |
|---|---|---|---|
| DBT | 1.58 | 4.30 | 2.68 |
| DBN | 4.25 | 6.16 | 1.53 |
| Ac | 3.27 | 5.24 | 1.65 |

### Energies of the excited electronic states of DBT

Energies and oscillator strengths for $S_1 \rightarrow S_i$ transitions of an isolated DBT molecule were calculated with the aid of the *ab initio* RHF CIS/3-21G (a convenient method is lacking in the frame of the TDDFT method included in Gaussian 09). It is well known that *ab initio* methods give larger values for the transition energies, thus the results of the CIS/3-21G calculations

included in Table S2 were scaled with factor 1.48. Such procedure led to quite good agreement between the $S_0 \rightarrow S_1$ transition energies calculated with the aid of both methods and describes well the experimental spectrum. An additional criterion for the sequence of states was their symmetry. Oscillator strengths for the $S_0 \rightarrow S_i$ transitions calculated by using the CIS/3-21G method were systematically bigger than the corresponding values obtained with the TDDFT/6-31G(d,p) method, but relations between different transitions are similar. Taking into account these observations, we note high oscillator strengths of the transitions $S_1$(Au)→$S_4$(Bg) and $S_1$(Au)→$S_7$(Ag), with the energies ~1.3 eV and ~1.5 eV, respectively. Our results are in agreement with the results of calculations described in the work of Sadeq *et al.*[S7] In conclusion, both states, $S_4$(Bg) and $S_7$(Ag), can be involved in the excitation from the $S_1$(Au) state, as proposed in our photoionization model which includes CT states (see below).

*Table 2. Energies of excited electronic states of DBT molecule and the oscillator strengths (f) for the $S_0 \rightarrow S_i$ [S8] and $S_1 \rightarrow S_i$ transitions.*

| | | TDDFT/B3LYP/6-31G(d,p) | | | CIS/3-21G | | | |
|---|---|---|---|---|---|---|---|---|
| | | $S_0 \rightarrow S_i$ | | $S_1 \rightarrow S_i$ | $S_0 \rightarrow S_i$ | | $S_1 \rightarrow S_i$ | |
| i | sym | ΔE [eV] | f | ΔE [eV] | ΔE [eV] | f | ΔE [eV] | f |
| 1 | AU | 1.584 | 0.383 | | 1.533 | 1.105 | | |
| 2 | BG | 2.601 | 0.000 | 1.017 | 2.583 | 0.000 | 1.049 | 0.022 |
| 3 | AG | 2.703 | 0.000 | 1.119 | 2.937 | 0.000 | 1.404 | 0.054 |
| 4 | BG | 2.872 | 0.000 | 1.288 | 3.012 | 0.000 | 1.479 | 0.640 |
| 5 | AU | 2.994 | 0.006 | 1.410 | 3.441 | 0.022 | 1.908 | 0.000 |
| 6 | BU | 3.087 | 0.010 | 1.503 | 2.760 | 0.011 | 1.227 | 0.000 |
| 7 | AG | 3.131 | 0.000 | 1.547 | 3.077 | 0.000 | 1.544 | 1.140 |
| 8 | AU | 3.267 | 0.201 | 1.683 | 3.159 | 0.157 | 1.626 | 0.000 |
| 9 | BG | 3.339 | 0.000 | 1.755 | 3.343 | 0.000 | 1.810 | 0.381 |
| 10 | BU | 3.354 | 0.012 | 1.770 | 3.288 | 0.021 | 1.755 | 0.000 |
| 11 | BU | 3.504 | 0.060 | 1.920 | 3.474 | 0.838 | 1.941 | 0.000 |
| 12 | BG | 3.593 | 0.000 | 2.009 | 3.700 | 0.000 | 2.166 | 0.046 |
| 13 | BG | 3.800 | 0.000 | 2.216 | 3.893 | 0.000 | 2.360 | 0.014 |
| 14 | BU | 3.844 | 0.418 | 2.260 | 3.995 | 0.231 | 2.462 | 0.000 |

## Calculations of locally excited (LE) and charge-transfer (CT) states

In this work, we make a distinction between two types of excited electronic states, which are characteristic for molecular solids and relevant for this work. The electronic excitation of a system with two or more molecules can lead to rearrangement of electronic charges between molecules, creating intermolecular electron transfers, or *charge-transfer (CT) states*. If such rearrangement of electron density happens intramolecularly, we talk about *locally excited (LE) states*. The electronic excited states may have also partially LE and partially CT character.

## Electronic states and transitions of bimolecular DBT/DBN system

*Table S3. TDDFT/B3LYP/3-21G results of energies and character of the electronic states in DBT/DBN system, calculated in the real crystal structure geometry of DBN. Red color in the energy levels diagram on the right indicates the contribution of CT character in the presented states. The states CT1 and CT3 are purely CT (DBT→DBN) states. The state CT2 has comparable contribution of the CT and LE characters. Electronic excitations $S_1$→CT2 and $S_1$→CT3, indicated by the red arrows, are supposed to contribute to the transfer of an electron from DBT to the nearby DBN molecule, leaving a hole on the DBT.*

| i | $\Delta E(S_0 \rightarrow S_i)$ [eV] | f | character of the dominant configuration of the electronic state |
|---|---|---|---|
| 1 | 1.823 | 0.428 | LE(DBT→DBT) |
| 2 | 2.667 | 0.001 | **CT1(DBT→DBN)** |
| 3 | 2.671 | 0.002 | LE(DBT→DBT) |
| 4 | 2.778 | 0.002 | LE(DBT→DBT) |
| 5 | 2.843 | 0.004 | LE(DBT→DBT) |
| 6 | 2.955 | 0.001 | BCT(DBN→DBT) |
| 7 | 3.030 | 0.029 | LE(DBT→DBT) |
| 8 | 3.252 | 0.013 | LE(DBT→DBT) |
| 9 | 3.279 | 0.008 | LE(DBT→DBT) |
| 10 | 3.375 | 0.090 | LE(DBT→DBT) |
| 11 | 3.428 | 0.100 | LE(DBT→DBT) |
| 12 | 3.462 | 0.021 | BCT(DBN→DBT) |
| 13 | 3.541 | 0.083 | LE(DBT→DBT) |
| 14 | 3.553 | 0.030 | LE(DBT→DBT) |
| 15 | 3.618 | 0.013 | **CT2(DBT→DBN)** |
| 16 | 3.819 | 0.001 | **CT3(DBT→DBN)** |
| 17 | 3.842 | 0.024 | LE(DBT→DBT) |
| 18 | 3.938 | 0.149 | LE(DBT→DBT) |

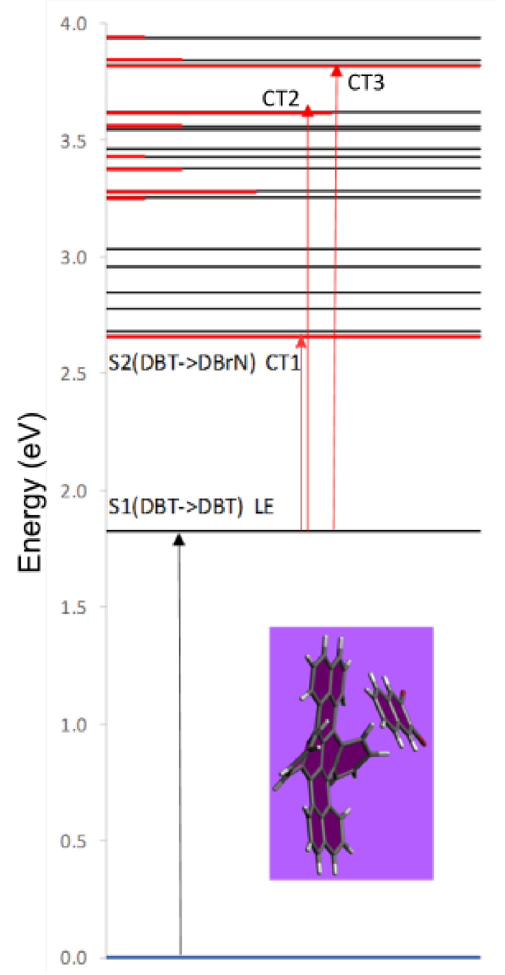


The lowest-energy electronically excited state of the DBT/DBN system, $S_1$, is localized on the DBT component. A sequence of two excitations which would be in agreement with the excitation energies applied in the experiment (~ 2.0 eV), goes as follows:

1. $S_0 \rightarrow S_1$(DBT), energy ~1.8 eV , and next
2. $S_1$(DBT) → $S_{15}$(CT2), $S_{16}$(CT3), $S_{17}$(LE), with excitation energy in range 1.8-1.9 eV.

Also, the nearby $S_{14}$ and $S_{18}$ states, attributed in Table S3 to LE states, have some contribution of CT character and thus may contribute to the electron transfer from DBT molecule to the surrounding DBN matrix. All these calculated transitions are within the excitation energy of the pump beam (~ 2 eV). High excitation powers are needed to excite a DBT molecule from the $S_1$ state to some higher electronic states with CT character, before the molecules relaxes back to the ground electronic state.

## Electronically excited states of DBT:Ac system

Electronically excited states of DBT/Ac system were calculated for two molecules, DBT and Ac, as well as for a DBT molecule surrounded by 4 molecules of Ac, arranged in the crystal geometry, as shown in Fig. S11. The results of calculations are collected in Table S4 and graphically presented in Fig. S11. The results for isolated DBT and Ac are also shown in Fig. S11 for comparison.

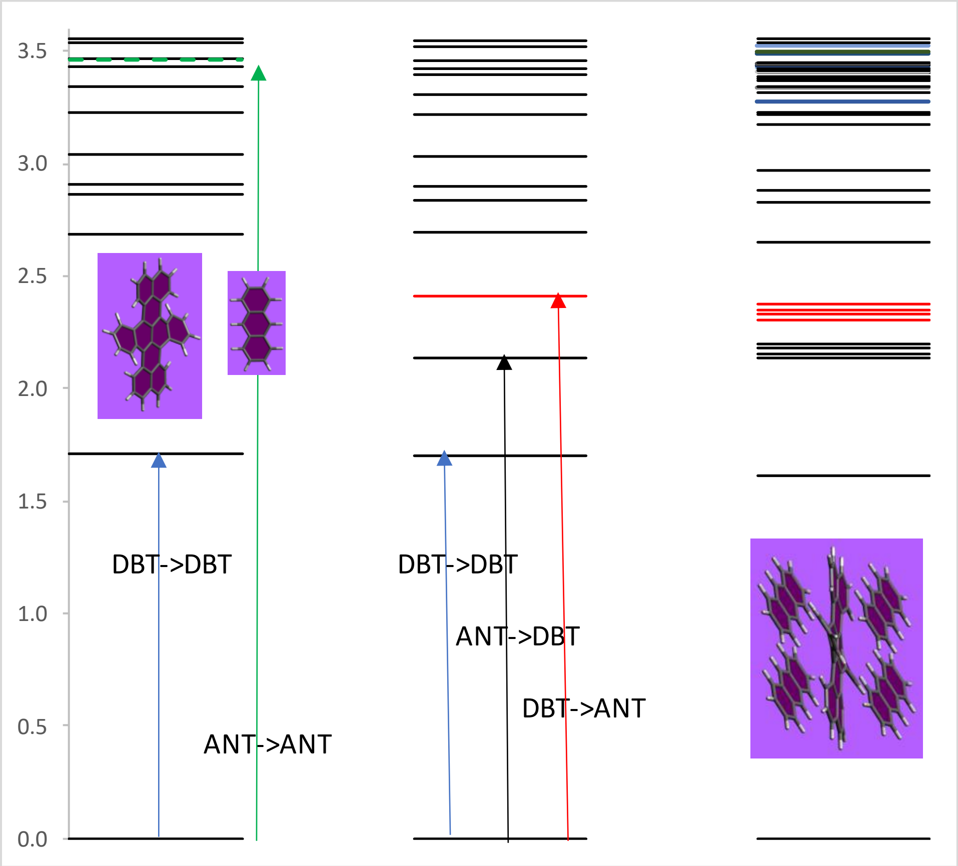


*Fig. S11. Diagrams of the electronic excited states of isolated DBT and Ac molecules (left), in the system composed of DBT molecule and one Ac molecule (center) and DBT surrounded by 4 molecules of Ac (right). Numerical data for DBT+4Ac are collected in Table S4.*

| Type of the dominant electronic configuration | ΔE [eV] | f |
|---|---|---|
| DBT→DBT | 1.618 | 0.281 |
| Ac→DBT | 2.139 | 0.029 |
| | 2.142 | 0.000 |
| | 2.188 | 0.000 |
| | 2.202 | 0.003 |
| DBT→Ac | 2.330 | 0.000 |
| | 2.335 | 0.000 |
| | 2.339 | 0.000 |
| | 2.377 | 0.014 |
| DBT→DBT | 2.654 | 0.000 |
| | 2.830 | 0.000 |
| | 2.885 | 0.000 |
| | 2.974 | 0.003 |
| | 3.178 | 0.001 |
| | 3.221 | 0.000 |
| Ac→Ac | 3.225 | 0.001 |
| | 3.227 | 0.001 |
| | 3.279 | 0.000 |
| | 3.281 | 0.003 |
| DBT→DBT | 3.320 | 0.033 |
| Ac→Ac | 3.341 | 0.000 |
| | 3.342 | 0.000 |
| *Ac→Ac DBT→DBT* | 3.369 | 0.148 |
| Ac→Ac | 3.379 | 0.000 |
| | 3.392 | 0.013 |
| | 3.403 | 0.000 |
| Ac→Ac Ac→DBT | 3.408 | 0.000 |
| | 3.413 | 0.013 |
| | 3.424 | 0.001 |
| DBT→DBT | 3.425 | 0.050 |
| Ac→Ac | 3.438 | 0.000 |
| | 3.444 | 0.006 |
| | 3.448 | 0.000 |
| | 3.450 | 0.003 |
| | 3.489 | 0.125 |
| Ac→DBT | 3.499 | 0.000 |

| | | |
|---|---|---|
| | 3.530 | 0.018 |
| | 3.539 | 0.000 |
| | 3.557 | 0.014 |
| | 3.613 | 0.000 |
| | 3.622 | 0.018 |
| | 3.683 | 0.006 |
| DBT→Ac | 3.689 | 0.000 |
| | 3.711 | 0.000 |
| | 3.760 | 0.059 |
| | 3.765 | 0.000 |
| | 3.776 | 0.021 |

*Table S4. Energies and oscillator strengths of electronic transitions in the system DBT+4Ac molecules. Different colors were used to distinguish transitions with different character. The „band" nature of the states, manifested by several states with similar energy, is a consequence of the presence of 4 Ac molecules.*

In the case of DBT/4Ac, the second photon, energy ~1.6 eV, following excitation of DBT molecule to its $S_1$ state (which is located 1.618 eV above the $S_0$), leads to the LE(DBT*) state of the energy 3.32 eV. This state is immersed in a dense distribution of excited states, described as Ac→Ac. In fact, we observed excited states where change of the distribution of charges following excitation concerns all 4 Ac molecules (see a visual example in Figure S12). Vibronic coupling leads to fluctuations of the energies of states, and, consequently, to their mixing. Charge-transfer dynamics was already modeled for the complex pentacene/C60 [S9], where it was based on the coupling of C−C bond-stretching and ring-breathings. Vibronic coupling between the LE(DBT*) and a manifold of (Ac→Ac) states can be considered as the reason of their mixing and evolution to the charge separated states.

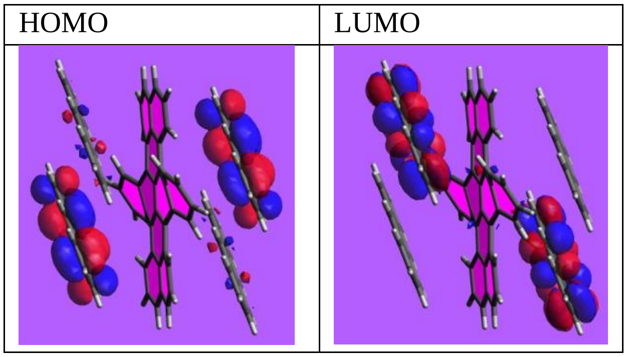


*Figure S12. HOMO and LUMO orbitals for the Ac→Ac transition with the energy 3.279 eV.*

The CT states between Ac molecules create charge carriers in Ac matrix, however we have not enough data to discuss this topic in more details.

## Recovery of neutral DBT

Upon excitation of DBT and subsequent electron ejection from DBT and charge transfer to a matrix molecule (DBN or Ac), the positively charged hole remains temporarily on DBT. We have considered the question of the energy barrier between $DBT^+$-Ac and DBT-$Ac^+$ and possibility of hole transfer from DBT to Ac. In this respect, there are two possibilities, i.e., spontaneous filling of the hole and recovery of neutral DBT with the aid of optical excitation.

### Case A: Spontaneous filling of the hole

Our calculations are analogous to polarization energy calculations in organic semiconductors [S10, S11], and the result is dependent on the number of host matrix molecules taken into consideration. Table S5 summarizes calculated energies for different numbers of Ac molecules in the unit cell.

*Table S5. Energies of the systems where DBT is surrounded by different numbers of Ac molecules. Calculations were done with the ONIOM (B3LYP/3-21G:B3LYP/3-21G) method.*

| Number of Ac molecules | E($DBT^+$-Ac) [au] | E(DBT-$Ac^+$) [au] | $\Delta$E [eV] |
|---|---|---|---|
| 1 Ac | -1988.3167 | -1988.2628 | 1.4652 |
| 4 Ac | -3598.0882 | -3598.0654 | 0.6217 |
| 36 Ac | -20764.8899 | -20764.8888 | 0.0299 |

The calculated energy difference in case of DBN–36Ac is small (~0.03 eV). Ionization potential in case of Ac molecule is smaller than the ionization potential of DBN. Similar calculations performed for DBT surrounded by molecules of DBN led to the energy barrier ~0.9 eV, an order of magnitude bigger than for Ac.

### Case B: Recovery of neutral DBT with the aid of optical excitation.

*Table S6. Energies of excitation for isolated cation of DBT with 1 molecule of DBN, and with 4 Ac molecules. Calculations performed with the TDDFT/B3LYP/3-21G method.*

| $DBT^+$ | | $(DBT\text{-}DBN)^+$ | | | $(DBT - 4\ Ac)^+$ | | |
|---|---|---|---|---|---|---|---|
| $\Delta$E [eV] | f | $\Delta$E [eV] | f | character | $\Delta$E [eV] | f | character |
| 0.927 | 0.092 | 1.061 | 0.006 | DBN→DBT | 0.472 | 0.000 | Ac→DBT |
| 1.706 | 0.062 | 1.245 | 0.031 | DBT→DBT | 0.479 | 0.000 | Ac→DBT |
| 1.913 | 0.256 | 1.523 | 0.010 | DBN→DBT | 0.583 | 0.022 | Ac→DBT |
| | | 1.562 | 0.019 | DBT→DBT | 0.600 | 0.000 | Ac→DBT |
| | | 1.807 | 0.347 | DBT→DBT | 1.102 | 0.055 | DBT→DBT |
| | | 1.865 | 0.027 | DBT→DBT | 1.658 | 0.054 | DBT→DBT |
| | | | | | 1.774 | 0.000 | Ac→DBT |
| | | | | | 1.778 | 0.046 | Ac→DBT |
| | | | | | 1.866 | 0.084 | Ac→DBT |

| | | | | | |
|---|---|---|---|---|---|
| | | | 1.875 | 0.000 | Ac→DBT |

In a range of small energies, comparable to the energies of excitation used in the experiment, there are CT transitions, where an electron is transferred from Ac or DBN to DBT.

1.523 eV in the system $DBT^{+}$-DBN

1.778 eV in the system $DBT^{+}$-4Ac

These results suggest that recovery of neutral DBT happens with the aid of optical excitation.

## Consistency of the model with experiments

We verify the consistency of our model with the following experimental observations:

- Illumination by the pump laser shifts the ZPLs almost continuously, and by up to several tens of GHz, with no significant broadening of the optical transition. This is consistent with our hypothesis that charges are trapped relatively far from the probed DBT molecule, so that each single-charge process gives rise to an undetectably small shift of the probed ZPL. The measured shift must result from the accumulation of many single-charge events at relatively large distances.
- The ZPL shift persists for long times, at least 24 h after the pump laser has been switched off. This indicates that the separated charges are far enough from each other that recombination by tunneling remains negligible on hours to days time scales. Such time scales require distances larger than tens of nm.
- The ZPL shift scales sub-linearly with power and can be fitted with a power law of time (eq. 1 of the main text). Power-law kinetics have been observed in the relaxation of charge distributions injected by electrodes in anthracene-based FETs [S12]. This observation supports our assignment of the ZPL shift to slowly varying charge distributions.
- The shift depends only weakly on the pump laser wavelength, with no clear effect of a resonance with DBT levels. This observation supports our assignment to a broad absorption or action spectrum, such as those of excited-state or molecular-ion absorption.
- The shift is observed both on dielectric and metallic substrates, indicating that the charge separation and trapping processes happen in the molecular material itself. The charges are not injected from non-organic materials outside the matrix.

The single-molecule time traces of resonant DBT molecules (Fig. 1 and Fig. 2.) give important hints as to local charge dynamics and electric fields. Instead of large discrete spectral jumps, the resonant DBT emitters appear to be continuously shifted for long periods of time by pump exposure. This suggests that many charge carriers contribute to the shift and that the separated charges do not reside in a close proximity of the probed DBT molecules. Furthermore, the long-

term stability of the spectral lines after pump illumination points toward long recombination times and low tunneling rates of the charge carriers trapped in the matrix. Assuming the low tunneling rates, we can estimate a lower bound to the distance between separated charges of at least 20 nm.

We first considered direct two-photon excitation of matrix molecules (Ac and DBN) as the possible photoionization mechanism. However, the close-to-linear power dependence of the frequency shift, shown in Fig. 2a, rules out single-step, two-photon-induced photoionization of the matrix. In both types of crystals, we observe background fluorescence whose spectrum shows that it originates from the pump-excited, non-resonant DBT molecules. This background also scales linearly with the excitation power (see SI). Finally, by using linearly polarized pump excitation on a well-oriented DBT:DBN single crystal, we verified that the intensity of the background fluorescence signal correlates with the magnitude of the spectral shift. As DBT cannot be ionized by a single pump or probe photon, we propose that DBT must be ionized via a cascade of two successive single-photon excitations (step A in Fig. 5). Photoionization results in two charged molecules, $DBT^+$ and $M^-$ (step B in Fig. 5). This charge-separated state most likely does not exist for long periods of time. Under conditions of strong illumination, however, both the trapped electron and the hole on DBT are likely to migrate further away into the matrix, creating thus $M^-$ and $M^+$ species with large separations. This conclusion is in line with our experimental observations. The latter step of photoinduced hole transport regenerates DBT to a photoactive state that can generate further separated electron-hole pairs (step C in Fig. 5).

Charge separation in the matrix is most likely induced by several background chromophores. These are found in large amounts in the densely doped DBT:DBN crystal, but also in small numbers in the DBT:Ac NCX, e.g. most likely embedded at the nanocrystal surfaces or at imperfections. These background molecules probably exhibit broad optical transitions, thus do not readily appear in high-resolution spectra, and do not significantly affect the anti-bunching measurements (see SI). Because these molecules are not necessarily resonant with the probe and probably give rise to very broad optical lines, the process is expected to be nearly independent of the pump frequency, as shown in Fig. 2c.

The ZPL spectral shits can be fitted with power laws, with a faster initial change that slows down in time (Figure 2). The spectral shift over time was also explained as consequent to charge transport in the guest-host system [S13]. Similar power-law behavior was reported for co-sublimated DBT:Ac crystals [S12], in the presence of hole injection by gold electrodes in contact with the anthracene crystal. These authors observed that charges initially trapped inside the crystal were subsequently de-trapped via migration in the host matrix and tunneling through the dielectric substrate (or via simple charge recombination through a metallic substrate). The similar kinetics in both cases suggests that dispersive transport in the organic matrix is at work in both cases.

It is worth noting that, during the pump illumination, we sometimes do observe small spectral jumps giving rise to noise on top of the power-law trend. These stochastic fluctuations of static

electric field might indicate discrete charge hopping events and therefore give an idea of their distance from the probed DBT molecule.

We have also considered other possible mechanisms that may take place during intense laser illumination. While light-induced single-molecule frequency shifts have already been reported in the literature [S14], the reported relatively weak shifts of about 600 MHz/W were reversible, non-tunable in time, and obtained under significantly stronger pump illumination. The authors ascribed the results to the combination of the beam absorption and ac-Stark effect [S15]. However, tunable all-optical frequency shifts of single molecules, which persist long after switching off of the pump source, have never been reported for single-photon emitters.

## Supplementary references


[S1] S. Pazzagli, P. Lombardi, D. Martella, M. Colautti, B. Tiribilli, F. S. Cataliotti, C. Toninelli, ACS Nano 2018, 12, 4295–4303.

[S2] R. C. Schofield, K. D. Major, S. Grandi, S. Boissier, E. A. Hinds, A. S. Clark, J. Phys. Commun. 2018, 2, 115027.

[S3] A. Nicolet, P. Bordat, C. Hofmann, M.A. Kol'chenko, B. Kozankiewicz, R. Brown and M. Orrit, *Single dibenzoterrylene molecules in an anthracene crystal. Main insertion sites*, ChemPhysChem 8 (2007) 1929-1936.

[S4] A. Moradi, Z. Ristanovic, M. Orrit, I. Deperasińska, B. Kozankiewicz, *Matrix-induced Linear Stark Effect of Single Dibenzoterrylene Molecules in 2,3-Dibromonaphthalene Crystal*, ChemPhysChem (2019)

[S5] N. Karl, Festkörperprobleme IX 1974, 261–290.

[S6] E. A. Silinsh, Organic Molecular Crystals: Their Electronic States, Springer, 1980.

[S7] Z. S. Sadeq, Rodrigo A. Muniz, and J. E. Sipe, Phys. Rev. Materials **2**, 075202 (2018).

[S8] A. Nicolet, C. Hofmann, M. Kol'chenko, B. Kozankiewicz, and M. Orrit, *Single dibenzoterrylene molecules in an anthracene crystal. I. Spectroscopy and photophysics*, ChemPhysChem 8 (2007) 1215-1220.

[S9] S. Joseph, M. Kumar Ravva, and J.-L. Bredas, *Charge-Transfer Dynamics in the Lowest Excited State of a Pentacene−Fullerene Complex: Implications for Organic Solar Cells*, J. Phys. Chem. Lett. 2017, **8**, 5171−5176.

[S10] J. E. Norton, J.-L. Bredas, *Polarization Energies in Oligoacene Semiconductor Crystals*, J. Am. Chem. Soc. 2008, **130**, 12377–12384.

[S11] F. Castet, P. Aurel, A. Fritsch, L. Ducasse, D. Liotard, M. Linares, J. Cornil, and D. Beljonne, *Electronic polarization effects on charge carriers in anthracene: A valence bond study*, Phys. Rev. B, 2008, **77**, 115210.

[S12] Nicolet, A. A. L., Kol'chenko, M. A., Hofmann, C. Kozankiewicz, B. & Orrit, M. Nanoscale probing of charge transport in an organic field-effect transistor at cryogenic temperatures. Phys. Chem. Chem. Phys.15, 4415–4421 (2013).

[S13] Scher, H. & Montroll, E. W. *Anomalous transit-time dispersion in amorphous solids*, Phys. Rev. B12,2455–2477 (1975).

[S14] Plakhotnik T., Walser D., Renn A. & Wild U. P., Light induced single molecule frequency shift, Phys. Rev. Lett. **77**, 5365–5368 (1996).

[S15] P. Tamarat, B. Lounis, J. Bernard, M. Orrit, S. Kummer, R. Kettner, S. Mais, T. Basché, Phys. Rev. Lett. 1995, 75, 1514–1517.
